# Supplementary material for: REFINE: Enhancing Program Repair Agents through Context-Aware Patch Refinement
Source: arXiv:2510.03588 source file (2025-10-04)
Supplement: Supplementary file 1 [file appendix.tex]

\appendix

\section{Appendix}
\label{sec:appendix}

\subsection{Modifications To The Reproducer}
\label{appendix:reproducer}

SpecRover contains a Reproducer Agent that takes in the issue description and generates a standalone python file that when executed in the repository reproduces the issue. The generated reproducer is determined to be successful if it raises an Assertion Error and exits with a non zero code with the prompt generating the reproducer specifically mentioning these conditions. In our experiments we have noticed that this system exit sys.exit() usually in a caught error can return stack traces that aren't helpful in localizing the faulty issues. We first improve the feedback prompt to specifically mention if a reproducers stack trace doesn't have an assertion error or exits with a zero code which significantly speeds up how many rounds it takes to generate a successful reproducer.

Next we add another component that takes in the best possible reproducer and runs it through an execution feedback loop with the goal of refining the reproducer and modifying it generate a more useful stack trace that can better help with issue localization. The feedback loop consists of passing the reproducer, the stack trace and the issue to the LLM and prompt it using a custom prompt that focuses on refining the reproducer to - (1) better reproduce the issue and (2) to remove potential try catch, system exit codes and assertion errors and generate a reproducer that gives the most detailed stack trace errors and incorporate an LLM call that decides if the stack trace is sufficiently useful or not. 

We find that this step significantly improves the quality of stack trace errors produced and constitutes the first step of our execution semantics.

\subsection{Identification of Suspicious Files From the Execution Trace}
\label{appendix:trace}

Once we have this refined reproducer, we run it and process the execution trace to identify all the relevant files that were called in the reverse order of contact i.e, the first file in the trace is the file that was last used before the crash occurred. We then identify all the files in the repository and store them in a set. Next we filter out the files obtained from the execution trace an only include those files that are both in the execution trace as well as in the repository, this gives us an ordered list of suspicious files that were last used when the crash happened. 

We then take the top 7 files and give this to the localization agent along with a prompt explaining why they are relevant. This is the second step in the execution semantics. The final step is running Spectrum-based Fault Localization and obtaining the top 5 most suspicious functions along with their class and file and sending this to the localization agent with a suitable prompt that similarly explains why these files are useful and how they were obtained.

\subsection{Repair Stage Caching}
\label{appendix:cache}

When the repair stage is executed for a given issue (\textit{I}) on a buggy file (\textit{F}) using an initial patch (\textit{P}), it produces a set of candidate patches (\textit{$p_i$}). We store these results in a cache, using the tuple (\textit{I}, \textit{F}, \textit{P}) as the key and the resulting patches (\textit{$p_i$}) as the value. This caching mechanism helps avoid redundant repair runs for previously encountered inputs, leading to significant cost savings. The cache is intended to be used primarily when running powerful models with temperature set to 0, to minimize variance. Use of the cache is \textbf{entirely optional} and was solely designed to help reduce cost.

\subsection{Prompts Used:}
\label{sec:prompts_used}

\begin{tcolorbox}
    [title={Generic System Prompt for Issue Semantics, Workflow generation, Context Retrieval and Fix Generation}]
You are a software developer working on fixing an issue in your code base. Another software developer has looked into this issue and has given 
a fix that solves the main issue or solves it to the best of the developers ability. Now, your goal is to analyze the possible call chains in a flle, go through and analyze them 
and determine if any additional changes need to be made in addition to the main change to maintain consistency in the code base while 
also fixing any edge cases or existing functionality that might have broken.
\end{tcolorbox}

\begin{tcolorbox}
[title={Prompt To Generate Issue Semantics}]
The issue might show a very specific example failing or not clearly explain the intent of the developer,  your goal is to understand the exact intent of what the issue conveys, and explain if this issue is part of a broader issue and if it is generalizable, and explain what the code should reflect to solve this issue as a whole,  then summarize everything you've said. Finally end it by by giving a paragraph that would direct an AI agent to fix changes that need to be made in the code base,  be as general as possible. The given issue you need to generalize is: "\{\textcolor{blue}{issue statement}\}". The final paragraph that directs an AI agent  should be in a <directions> ... </directions> block.
\end{tcolorbox}

\begin{tcolorbox}
[title={Prompt To Generate Workflows}]
    You are an AI assistant trying to solve an issue: \{\textcolor{blue}{issue semantics}\}, you have correctly figured out the main buggy file and fixed it using the 
        patch: "\{\textcolor{blue}{initial patch}\}" you however miss other changes required to maintain the consistency of the fix throughout the file. the content of the 
        file: "\{\textcolor{blue}{buggy file name}\}" is: "\{\textcolor{blue}{code in buggy file}\}". Your task is to figure out the different flows of execution of the file along with the names of the methods called.
        We will then look at each execution flow and determine if there needs to be other fixes in addition to the main fix to maintain consistency.\\
\\
        Each flow must be in the following format: \\ \\
        <flow> \\
        <step> describe the approach...</step> \\
        <step> ... </step> \\
        ... \\
        </flow> \\

        <flow> \\
        <step>...</step> \\
        <step>...</step> \\
        ... \\
        </flow> \\
\\
        ...\\
\\
        Each flow much be encased in <flow> </flow> and each step must be in <step> </step>. \\
\end{tcolorbox}

\begin{tcolorbox}
    [title = {Prompt To Get Relevant Context For A Step}]
    You are analyzing a call chain, and are given steps that describe steps in a flow such as `\_read\_table\_qdp()` calls `\_get\_tables\_from\_qdp\_file()`,
        along with the entire code in the file that the call chain resides in. Your goal is to understand the relevant code snippets that need to be 
        extracted in order to analyze this step and solve an issue. Your output should be a JSON with the key describing the code snippet, and the 
        value being the code in the code snippet. NOTE: If you are giving the code of a method then you must give the ENTIRE code in the method. Also note that the key and values of the JSON must be strings.
        For example, for the `\_read\_table\_qdp()` calls `\_get\_tables\_from\_qdp\_file()` step, the key should be something like "code in the \_get\_tables\_from\_qdp\_file() method",
        and the value should be the code in the \_get\_tables\_from\_qdp\_file method.
        the resulting JSON structure should look like:
        {{
            "code in the \_get\_tables\_from\_qdp\_file() method": Get all tables from a QDP file.  Parameters .... (rest of the \_get\_tables\_from\_qdp\_file method code)
        }}
        The file\_content is: "\{\textcolor{blue}{File Content}\}", and the step in the call chain is: "\{\textcolor{blue}{Step}\}".
        Your goal is to find the relevant code snippets as mentioned above.
        NOTE: Try to focus the majority at a method level of granularity, however you can also use a class level or expression level of granularity.
        This information will be given to another AI agent who will suggest code changes to fix the bug and maintain consistency throughout the file.
\end{tcolorbox}

\begin{tcolorbox}
[title={Prompt To Generate Fixes}]
    You are given an execution 
            flow: <flow>"\{\textcolor{blue}{Flow} \}"</flow> and general directions on how to fix it: <directions>" {Issue Semantics} "</directions>. In this flow we focus on the step: <step>""\{\textcolor{blue}{Step}\}"</step>
            .the relevant code snippets are: <codesnippets>""\{\textcolor{blue}{Relevant Code Snippets}\}"</codesnippets>, and another AI agent has given an initial patch: <patch>""\{\textcolor{blue}{Initial Patch}\}"</patch> that could potentially have solved the bulk of the issue. Your goal is to analyze these code snippets and identify changes that need to be made to maintain consistency 
            with the general directions provided to solve the overall issue. 
            These can be minor or major changes that try to maintain consistency in the file, 
            fix edge cases that might have been missed, 
            or fix modified code that might break important existing functionality. 
            Please be EXTREMELY thorough, go through each line of context given to make 
            sure that you have not missed anything that needs to be changed. You can give your reasoning, however your final changes must be in 
            <changes>...</changes> angle brackets, with the original code, patched code and reasoning, preferably in a <original>...</original> 
            <patched>...</patched> <reason>...</reason> format. If there are no changes to be made then the output must be "No changes" in the angle brackets, 
            i.e <changes>No changes</changes>.
            
\end{tcolorbox}

\newpage

\begin{tcolorbox}[breakable, title = {Prompt For Repair Stage Fixes Reviewer}]
\textbf{System Prompt:}\\ \\
You are an expert software code reviewer who evaluates suggestions made by multiple software engineers attempting to solve a specific issue in a code file.\\

Your role is to:\\
- Understand the issue in depth.\\
- Analyze each suggestion carefully, identifying which are necessary, which are helpful, and which may be incorrect or unnecessary.\\
- Apply clear and well-reasoned judgment to select the best combination of suggestions to fully and correctly resolve the issue.\\

You prioritize correctness and consistency in your review. Use precise reasoning when justifying your decisions.\\

\textbf{User Prompt:}\\\\
You are reviewing and trying to solve the following issue in a code file:

        <issue> "\{\textcolor{blue}{Issue Statement}\}" </issue>\\

        The full content of the file is:\\

        <file content> "\{\textcolor{blue}{File Content}\}" </file content>\\

        A number of software engineers have provided suggestions, each aiming to solve the issue along with a starting fix to build on that most likely fixes the bulk of the issue:\\

        <starting fix> "\{\textcolor{blue}{Patch Content}\}" \\</starting fix>\\

        These suggestions consist of the original code, the patched code, and the reasoning for why this change was suggested.
        Your goal is to filter out unnecessary suggestions while keeping the useful ones.\\

        Useful suggestions fall into one of these categories:\\
        - Suggestions ensuring the consistency of the fix throughout the file.\\
        - Suggestions identifying edge cases that might have been missed by the starting fix.\\
        - Suggestions fixing code that may have been broken by the starting fix.\\
        - Suggestions that solve the core issue if the starting patch identifies a wrong fix.\\

        where as,\\
        
        Unnecessary suggestions fall into one of these categories:
        - Changes that break existing functionality. Use your best judgment when deciding this.\\
        - The addition of unnecessary try catch statements or assertions which look good in theory but are unnecessary as they might break unit testing for that particular functionality and could have already been caught else where.\\
        - If the issue is incredibly simple to fix, then avoid overtly complex suggestions which are prone to break some existing functionality.\\

        You will be given "\{\textcolor{blue}{Number of Patches}\}" suggestions in the format of:\\
        
        0: <original> ... </original> <patched> ... </patched> <reason> ... </reason>\\
        1: <original> ... </original> <patched> ... </patched> <reason> ... </reason>\\ \\
        and so on, with 0: representing the 0th patch, 1: the 1st, etc...\\

        Your output must be a JSON object in the following format:
\\
        \{\{ \\
            "0": \{\{ \\
                "reason": "Explanation of why this suggestion is necessary or not.", \\
                "required": "Required or Not Required", \\
            \}\}, \\
            "1": \{\{ \\
                "reason": "Explanation of why this suggestion is necessary or not.", \\
                "required": "Required or Not Required", \\
            \}\}, \\
            ... \\
        \}\} \\
\\
        - Each key corresponds to the suggestion ID. \\
        - The "reason" field must contain a concise, clear justification for why the suggestion is necessary or not. \\
        - The "required" field should be `Required` if the suggestion is required to solve the issue, or `Not Required` if it is not needed. \\
        - Always begin with your reasoning in the "reason" field, followed by the decision in the "required" field. \\

        The suggestions are: \\

        "\{\textcolor{blue}{Patches Enumerated One By One}\}" \\

        If there are no suggestions then return None.
        """

\end{tcolorbox}

% \section{Research Methods}

% \subsection{Part One}

% Lorem ipsum dolor sit amet, consectetur adipiscing elit. Morbi
% malesuada, quam in pulvinar varius, metus nunc fermentum urna, id
% sollicitudin purus odio sit amet enim. Aliquam ullamcorper eu ipsum
% vel mollis. Curabitur quis dictum nisl. Phasellus vel semper risus, et
% lacinia dolor. Integer ultricies commodo sem nec semper.

% \subsection{Part Two}

% Etiam commodo feugiat nisl pulvinar pellentesque. Etiam auctor sodales
% ligula, non varius nibh pulvinar semper. Suspendisse nec lectus non
% ipsum convallis congue hendrerit vitae sapien. Donec at laoreet
% eros. Vivamus non purus placerat, scelerisque diam eu, cursus
% ante. Etiam aliquam tortor auctor efficitur mattis.

% \section{Online Resources}

% Nam id fermentum dui. Suspendisse sagittis tortor a nulla mollis, in
% pulvinar ex pretium. Sed interdum orci quis metus euismod, et sagittis
% enim maximus. Vestibulum gravida massa ut felis suscipit
% congue. Quisque mattis elit a risus ultrices commodo venenatis eget
% dui. Etiam sagittis eleifend elementum.

% Nam interdum magna at lectus dignissim, ac dignissim lorem
% rhoncus. Maecenas eu arcu ac neque placerat aliquam. Nunc pulvinar
% massa et mattis lacinia.
